# Supplementary material for: N-GCN: Multi-scale Graph Convolution for Semi-supervised Node Classification
Source: arXiv:1802.08888 source file (2018-02-24)
Supplement: Supplementary file 1 [file appendix.tex]

\newpage
\section{Appendix}
\subsection{Algorithm for Network of SAGE}
Algorithms \ref{alg:sage} and \ref{alg:nsage}, respectively, define SAGE \cite{sage} and Network of SAGE (N-SAGE). 
Algorithm \ref{alg:sage} assumes mean-pool aggregation by \cite{sage}, which performs on-par to their top performer max-pool aggregation. Further, Algorithm \ref{alg:sage} operates in full-batch while \cite{sage} offer a stochastic implementation with edge sampling. Nonetheless, their proposed stochastic implementation should be wrapped  in a network, though we would need a way to approximate (e.g. sample entries) from dense $\hat{A}^k$ as $k$ increases. We leave this as future work. 

\begin{figure*}[h]
	\begin{minipage}[t]{2.8in}
		\begin{algorithm}[H]
			\caption{SAGE Model \citep{sage}} 
			\label{alg:sage} 
			\begin{algorithmic}[1]
				\Require{$\hat{A}$ is a normalization of $A$}
				\Function{SageModel}{$\hat{A}$, $X$, $L$}
				\State {$Z \leftarrow X$}
				\For{$i = 1 $ to $L$}
				\State{$Z \leftarrow \sigma(\left[ \begin{array}{c;{2pt/2pt}c}
					Z & \hat{A} Z
					\end{array} \right] W^{(i)})$ }
				\State{$Z \leftarrow \textsc{L2NormalizeRows}(Z)$ }
				\EndFor
				\State{\Return $Z$}
				\EndFunction
			\end{algorithmic}
		\end{algorithm}
	\end{minipage}
	\hfill
	\begin{minipage}[t]{2.8in}
		\begin{algorithm}[H]
			\caption{N-SAGE} 
			\label{alg:nsage} 
			\begin{algorithmic}[1]
				\Function{Nsage}{$A$, $X$}
				\State{$D \leftarrow \textbf{diag}(A \mathbf{1}) $}
				\Comment{Sum rows}
				\State{$\hat{A}  \leftarrow D^{-1}A$}
				\State{\Return $\textsc{Network}(\textsc{SageModel}, \hat{A}, X, 2)$}
				\EndFunction
			\end{algorithmic}
		\end{algorithm}
	\end{minipage}
	\hfill
\end{figure*}

Using SAGE with mean-pooling aggregation is very similar to a vanilla GCN model but with three differences. First, the choice of adjacency normalization ($D^{-1}A$ versus $D^{-\frac{1}{2}}AD^{-\frac{1}{2}}$). Second, the skip connections in line 4, which concatenates the features with the adjacency-multiplied (i.e. diffused) features. We believe this is analogous in intuition of incorporating $\hat{A}^0$ in our model, which keeps the original features. Third, the use of node-wise L2 feature normalization at line 5, which is equivalent to applying a layernorm transformation \cite{layernorm}. Nonetheless, it is worth noting \cite{sage}'s formulation of SAGE is flexible to allow different aggregations, such as max-pooling or LSTM, which further deviates SAGE from GCN.

%\subsection{Sensitivity Analysis}

%Earlier, in Table \ref{table:results}, we showed the test performance corresponding to the model performing best on the validation split. The number of labeled nodes are small, and such model selection is important to avoid overfitting. For example, there can be  up to $10\%$ relative test accuracy difference when training the \textit{same} model architecture  but with \textit{different} random seed. In this section, we programatically sweep hyperparameters $r$, $K$, choice of classification network ($\in \{\textrm{fc}, \textrm{a}\}$), and whether or not we enable $\hat{A}^0$, for both N-GCN and N-SAGE models.

%The settings when ($K=1$, $r=1$, and $\hat{A}^0$ disabled), correspond to the vanilla base model. Further, the settings when ($K=1$, $r>1$, and $\hat{A}^0$ disabled), correspond to an ensemble of the base model. These cases are outperformed when $K>1$, showing that \textit{unmodified} random walks indeed help these convolutional methods perform better, by gathering information from nearby and distant nodes.

%The automatically generated tables are shown below:

%\input{sweep_tables.tex}

%\bibliography{appendix}
%\bibliographystyle{iclr2018_conference}
